# Supplementary material for: Retention Is All You Need
Source: arXiv:2304.03103 source file (2023-08-26)
Supplement: Supplementary file 1 [file supplementary.tex]

\section{Supplementary Material}
\subsection{Introducing Heatmap}
Features in attrition have a high dependency and affect each other.
We used a heatmap visualization of the features in order to understand the correlation among the features shown in \ref{fig:heatmap1}.
%This heatmap provides an idea which positive features could be the important factors in the prediction model. 
The correlation of the features in the heatmap are used as an additional indicator for the prediction. 
However, several features such as Over18, EmployeeCount, EmployeeNumber, and StandardHours have been dropped as they showed low impact in the correlation matrix.
%From this heatmap the assumption is to obtain the positively correlated features. 
For example, MonthlyIncome is highly correlated with feature Job Level which could be a useful insights.
\begin{figure}[H]
    \includegraphics[width=\linewidth]{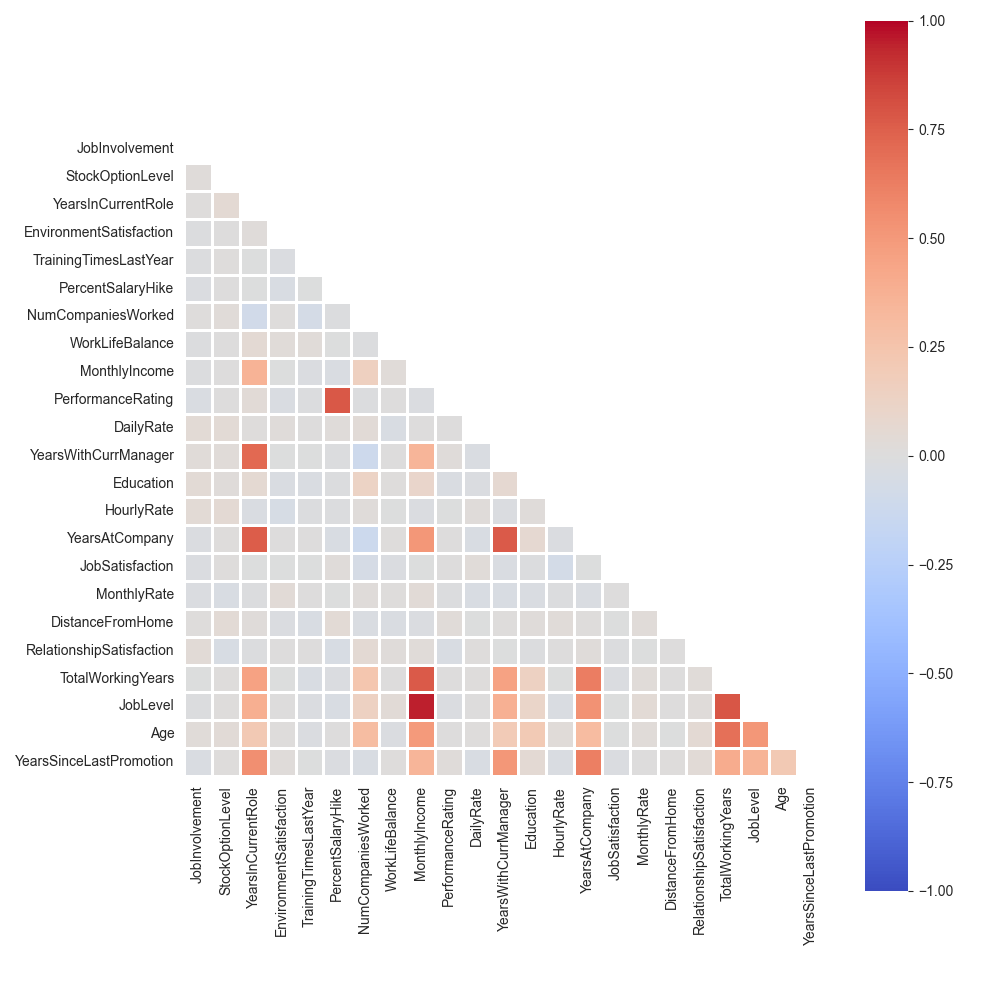}
     \caption{Correlation of the features in the IBM data.}
    \label{fig:heatmap1}
\end{figure}

\subsection{Confusion Matrix and AUC for XGB}
To evaluate accuracy of models using different approaches with XGB, we focused on evaluation with/without outlier, with/without added weight features.
We performed evaluation with regards to several metrics such as confusion matrix \ref{fig:confusion} and area under curve (AUC) \ref{fig:auc}.
Confusion metric shows that XGB with added feature weights is performing better than other models due to having less number of false positives (6) and negatives (26). 
The diagonal cells represent correct predictions i.e, true positives(249) and true negatives(13). 
Other cells represents incorrect predictions i.e, false positives and false negatives.
The first matrix on the left side is the results without using any methods. The second one in the left side shows the results with outlier detection technique.
The third one is using the added feature weights and the last one is using both techniques.
\begin{figure}[H]
%\centering
    \includegraphics[width=0.118\textwidth]{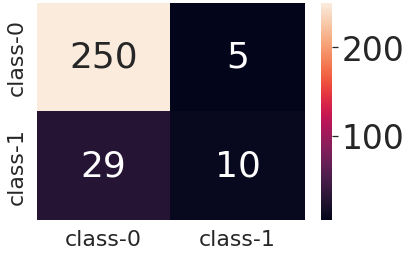}\hfill
    \includegraphics[width=0.118\textwidth]{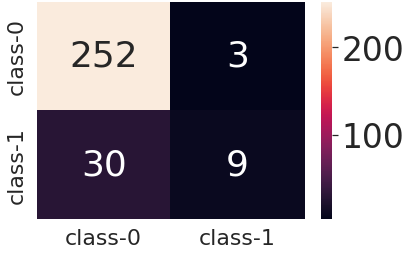}\hfill
    \includegraphics[width=0.118\textwidth]{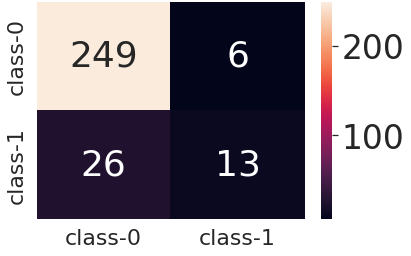}\hfill
    \includegraphics[width=0.118\textwidth]{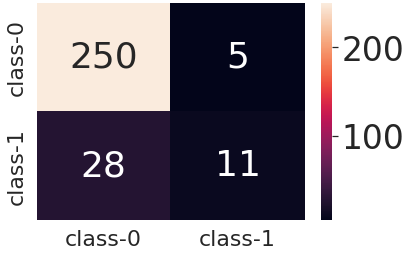}
     \caption{Confusion matrix of XGB algorithms is shown.}
     \label{fig:confusion}
\end{figure}

\begin{figure}[H]
%\centering
    \includegraphics[width=0.22\textwidth]{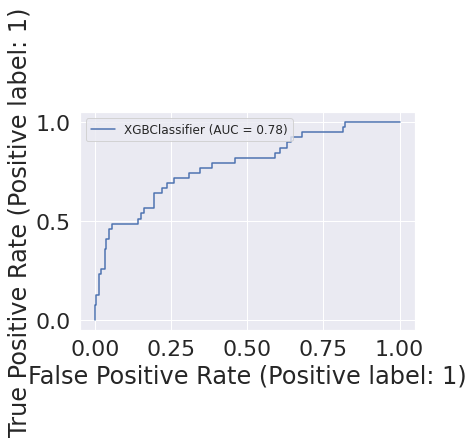}\hfill
    \includegraphics[width=0.22\textwidth]{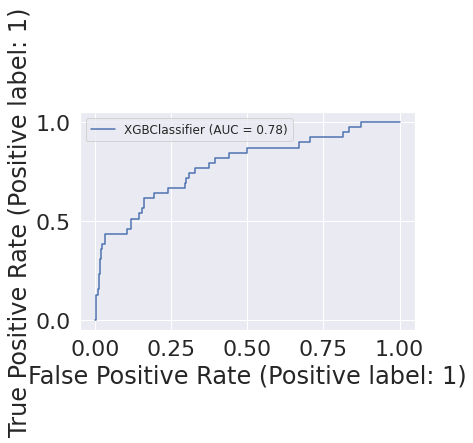}\hfill
    \includegraphics[width=0.22\textwidth]{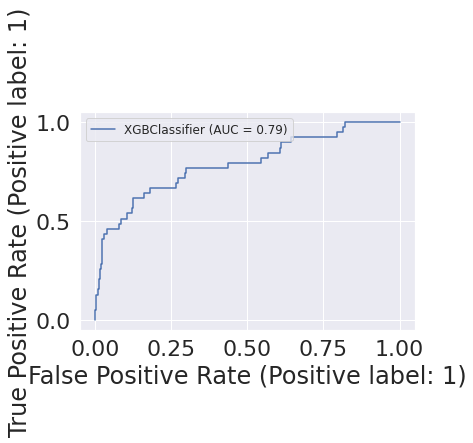}\hfill
    \includegraphics[width=0.22\textwidth]{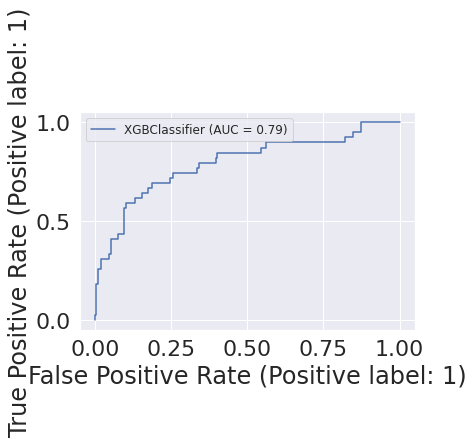}
     \caption{AUC of XGB algorithms.}
     \label{fig:auc}
\end{figure}

\subsection{SHAP Feature Importance} 
SHAP feature importance are measured by the mean of absolute Shapley values. 
The important features of the XGB model using Random Forest Classifier can be explained by observing the SHAP feature importance visualization. 
\begin{figure}
    \includegraphics[scale=0.22]{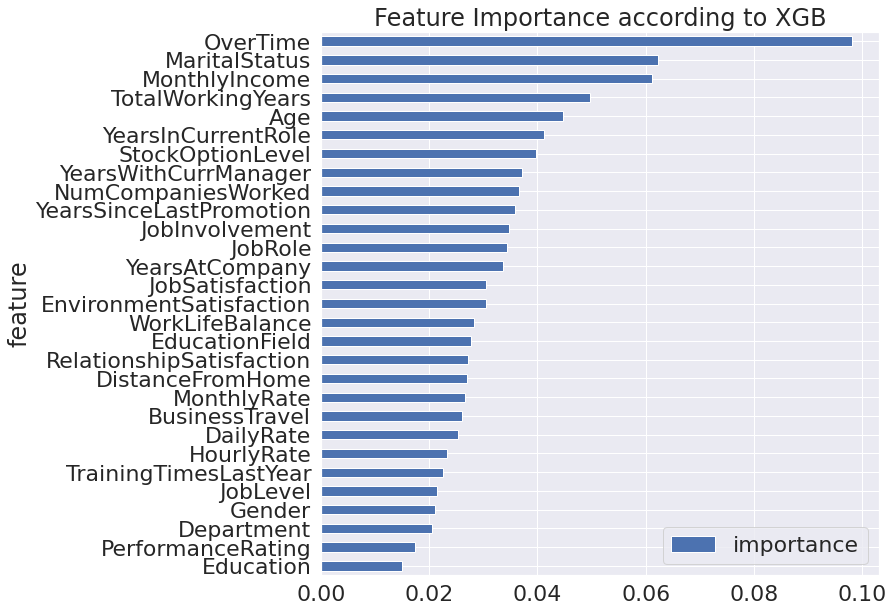}
     \caption{Top 30 feature importance by SHAP}
    \label{fig:ft}
\end{figure}
Figure \ref{fig:ft} illustrated the most significant features for employee attrition.
The feature importance are distributed in descending order, where the most significant feature is- 'OverTime', followed by 'MartialStatus' and 'MonthlyIncome' for attrition.
%There are 32 instances are wrongly predicted. For example, if we consider OverTime,
%\subsection{SHAP Summary Plot} 
%In addition, to investigate correct prediction, wrongly predicted instances are also observed in the summary plot in figure \ref{fig:wrong} for XGB with added weight features.
%\begin{figure}
%    \centering
%    \includegraphics[scale=0.35]{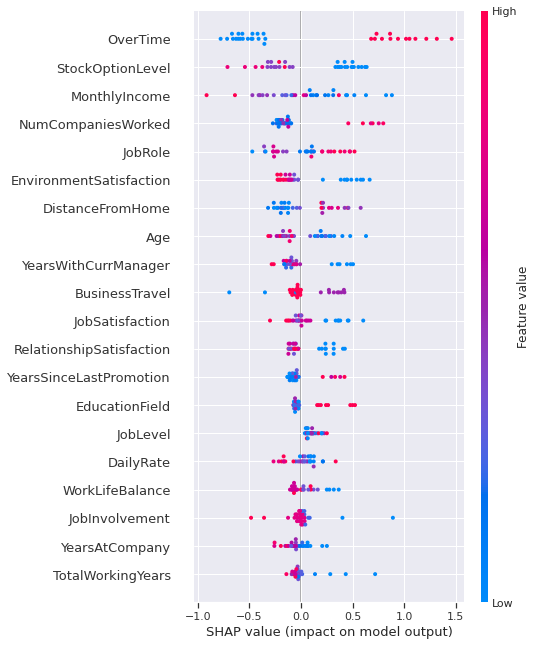}
%    \caption{Summary plot for incorrect predictions.}
%    \label{fig:wrong}
%\end{figure}
% \section{Online Resources}

% Nam id fermentum dui. Suspendisse sagittis tortor a nulla mollis, in
% pulvinar ex pretium. Sed interdum orci quis metus euismod, et sagittis
% enim maximus. Vestibulum gravida massa ut felis suscipit
% congue. Quisque mattis elit a risus ultrices commodo venenatis eget
% dui. Etiam sagittis eleifend elementum.

% Nam interdum magna at lectus dignissim, ac dignissim lorem
% rhoncus. Maecenas eu arcu ac neque placerat aliquam. Nunc pulvinar
% massa et mattis lacinia.

\end{document}
